# Supplementary material for: Classification based on invisible features and thereby finding the effect of tuberculosis vaccine on COVID-19
Source: arXiv:2011.07332 source file (2020-11-14)
Supplement: Supplementary file 1 [file AppendixTemplate.tex]

% Appendix Template

\chapter{Appendix Title Here} % Main appendix title

\label{AppendixX} % Change X to a consecutive letter; for referencing this appendix elsewhere, use \ref{AppendixX}

Write your Appendix content here.
